# Supplementary material for: Excited states of neutral and charged excitons in single strongly asymmetric InP-based nanostructures emitting in the telecom C band
Source: arXiv:2106.14695 ancillary file (2021-06-28)
Supplement: Supplementary file 1 [file supplemental.pdf]

# Supplemental Material: Excited states of neutral and charged excitons in single strongly asymmetric InP-based nanostructures emitting in the telecom C band

M. Gawełczyk,[1,2] P. Wyborski,[2] P. Podemski,[2] J. P. Reithmaier,[3] S. Höfling,[4,5] and G. Sęk[2]

[1]*Department of Theoretical Physics, Faculty of Fundamental Problems of Technology, Wrocław University of Science and Technology, 50-370 Wrocław, Poland*
[2]*Laboratory for Optical Spectroscopy of Nanostructures, Department of Experimental Physics, Faculty of Fundamental Problems of Technology, Wrocław University of Science and Technology, 50-370 Wrocław, Poland*
[3]*Institute of Nanostructure Technologies and Analytics (INA), CINSaT, University of Kassel, Heinrich-Plett-Str. 40, 34132 Kassel, Germany*
[4]*Technische Physik, University of Würzburg and Wilhelm-Conrad-Röntgen-Research Center for Complex Material Systems, Am Hubland, D-97074 Würzburg, Germany*
[5]*SUPA, School of Physics and Astronomy, University of St.Andrews, North Haugh, KY16 9SS St. Andrews, United Kingdom*

In this Supplemental Material, we present a detailed analysis of single-QD family of carrier complexes as well as additional examples of measured μPLE traces along with simulated absorption spectra that, within our model, fit these data the best.

## EXCITATION-POWER DEPENDENCE OF EMISSION FROM CARRIER COMPLEXES

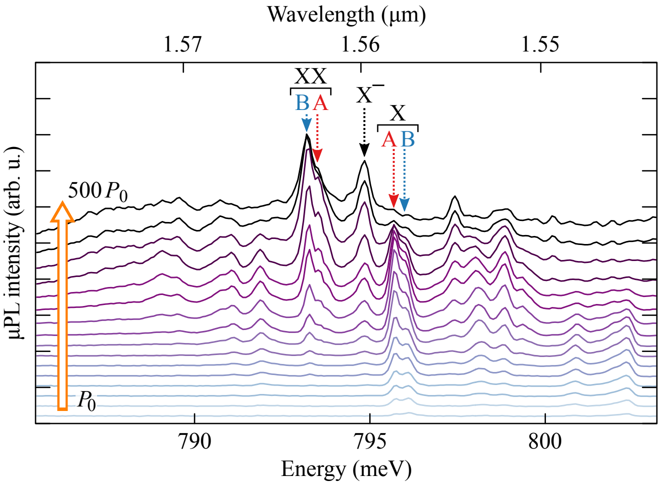


FIG. S1. Exictation-power series of μPL spectra. Lines chosen for analysis are marked with arrows.

Here, we focus in more detail on the family of lines from Fig. 1 (of the main text) marked with labels: XX, $X^-$, A, and B. Based on the polarization of their emission as well as excitation-power dependence of their intensity, these are identified as coming from neutral biexciton, charged exciton and neutral-exciton fine structure, respectively. In Fig. S1, we present the relevant magnified part of μPL spectra taken under nonresonant CW excitation, while in Fig. S2 intensity of these lines versus pumping power is plotted with symbols. Fine structure split peaks are taken cumulatively. Basic distinction between single- and multi-exciton complexes can be made by checking the exponent $\alpha$ of the intensity power-law dependence, $I \propto P^{\alpha}$, on the excitation power $P$ in the weak-pumping regime. This is typically close to $\alpha = 1$ for X and 2 for XX, and in the range of 1-1.5 in the case of $X^-$. For the X-XX recombination cascade rate-equation models with

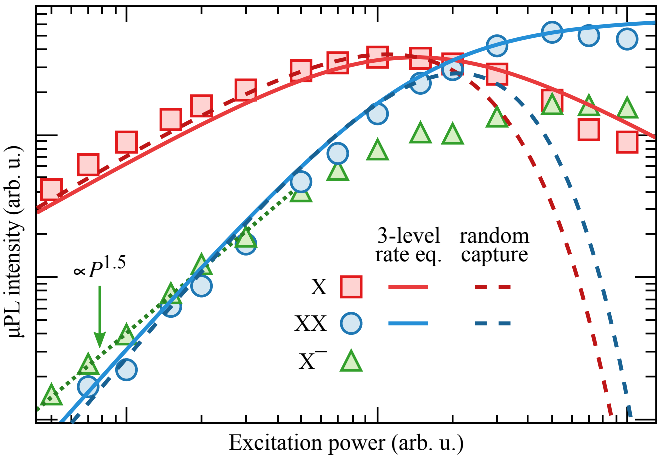


FIG. S2. Excitation-power dependence of luminescence intensity for lines marked in Fig. S1 (symbols) along with fits for the XX-X cascade obtained within the simple rate-equation (solid lines) and random capture (dashed) models. Dotted line marks a $\propto P^{1.5}$ dependece.

a few states are commonly used [1]. While originally developed for large ensembles of QDs, a modified random-capture rate-equation model [2] is sometimes applied also to emission from single dots [3]. In Fig. S2, we utilize both, and plot the fits with solid and dashed lines, respectively. While in the low-power regime the curves from two models agree, we notice a significant difference at higher powers. This comes from the fact that for the rate-equation model only 3 levels have been used, while the random-capture model comes without an upper limit for the number of excitons that may be generated in QDs. Including more levels (multi-exciton states) in the former would also lead to a more abrupt decrease of X and XX intensities at high power, as it happens in the random-capture model. However, this would not fit our data well, from which we draw a conclusion that bright multi-exciton complexes are generated with very low probability or are not formed at all, *i.e.*, the model including only the XX, X and vacuum states corresponds well to the actual kinetics occurring in the sys-

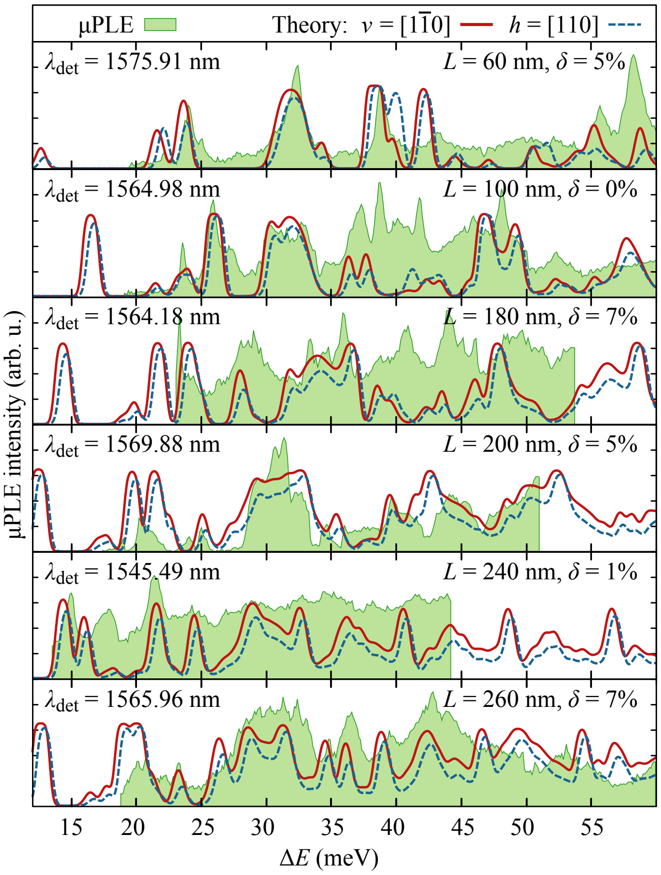


FIG. S3. µPLE spectra for various X lines (filled) and best fitting calculated polarization-resolved absorption spectra for QDs with given length $L$ and with bump characterized by $\delta$ (lines).

tem. The only meaningful free parameter in the three-level rate-equation model is $\tau_X/\tau_{XX}$, *i.e.*, the ratio of radiative life times of X and XX complexes. The presented lines correspond to $\tau_X/\tau_{XX} \simeq 1/2$, which is in line with expectations, as values below 1 are typical for QDs in the weak confinement regime [1]. Regarding the $X^-$ line, we find a close to $\propto P^{1.5}$ dependence in the weak pumping limit, which may indicate that the additional electron in the complex comes rather from optical excitation than from a reservoir of residual carriers. In the latter case a close to linear trend is typically found [3].

## ABSORPTION-LIKE SPECTRA: MEASURED µPLE AND SIMULATED ABSORPTION

To extend the presentation of results from the main paper, in Fig. S3 we show examples of µPLE traces from various mesas with QDs (filled curves), along with simulated absorption spectra for the neutral exciton that fit the data the best within our model (lines). At each panel, we give the emission wavelength, at which the experimental spectrum has been collected as well as parameters used in the calculation: QD length $L$ and bump size $\delta$.


[1] G. Sęk, A. Musiał, P. Podemski, and J. Misiewicz, On the applicability of a few level rate equation model to the determination of exciton versus biexciton kinetics in quasi-zero-dimensional structures, J. Appl. Phys. **108**, 033507 (2010).

[2] M. Grundmann and D. Bimberg, Theory of random population for quantum dots, Phys. Rev. B **55**, 9740 (1997).

[3] M. Abbarchi, C. Mastrandrea, T. Kuroda, T. Mano, A. Vinattieri, K. Sakoda, and M. Gurioli, Poissonian statistics of excitonic complexes in quantum dots, J. Appl. Phys. **106**, 053504 (2009).
